# Supplementary material for: Towards True Lossless Sparse Communication in Multi-Agent Systems
Source: arXiv:2212.00115 source file (2022-11-30)
Supplement: Supplementary file 1 [file 07_appendix.tex]

% \appendix{}
% \section{Appendix}

% % \subsection{Additional Experiments}
% % Budget adherence is motivated by methods maintaining sparsity over an entire episode, but observing issues with communication spikes during a subset of an episode \cite{benSparseDiscrete}. We show that the communication regularization term is able to prevent communication spiking. In Figure~\ref{fig:budget_adherance}, we analyze the average number of communications emitted by an agent over $t_\delta = 5$ time-steps. We observe that our model is able to adhere to the budget over periods within the episode as well as over the entire episode. We observe some small spiking behavior over the budget followed by a large dip, which derives from the small $t_\delta$.

% % \begin{figure}[!h]
% %     \centering
% %     \includegraphics[width=.45\textwidth]{figs/traffic_junction_False.png}
% %     \includegraphics[width=.45\textwidth]{figs/traffic_junctionhard_False.png}
% %     \includegraphics[width=.45\textwidth]{figs/traffic_junction_True.png}
% %     \includegraphics[width=.45\textwidth]{figs/traffic_junctionmed_True.png}
% %     \caption{Budget Adherence averaged over 5 time-steps within an episode. Our results show that our model is able to communicate within the budget over periods within the episode as well as overall.}
% %     \label{fig:budget_adherance}
% % \end{figure}

% % \subsection{Traffic Junction Setup}\label{tj_setup}

% % The traffic junction, which is composed of discretized cells, have specified entry cells and exit cells for spawning and leaving the environment. The agents spawn randomly with some specified probability at one of the entry cells and are assigned an exit cell randomly. The agents then navigate from their spawn cells to their exit cells along the shortest possible route while avoiding collisions. The agents can undertake two possible actions in the environment at every time-step: move or stop.

% % The ``easy'' variant of the traffic junction environment is a traffic intersection formed by two one-way roads. Furthermore, the ``easy'' variant maintains a maximum of 5 agents in the environment at any given time and the length of the environment is 7. 
% % The ``medium'' variant of the traffic junction environment is a standard four-way traffic intersection. Furthermore, the ``medium'' variant maintains a maximum of 10 agents in the environment at any given time and the length of the environment is 14. 
% % The ``hard'' variant of the traffic junction environment is composed of four connected standard four-way traffic intersections arranged as 4 corners of a square, similar to a block. Furthermore, the ``hard'' variant maintains a maximum of 20 agents in the environment at any given time and the length of the environment is 18. 

% % {See appendix for additional experiments - fully cooperative predator-prey}

% % For each of these variants, we train on 10 random seeds. The model was trained using 16 parallel processes, with each process using a batch size of 500. Concurrently training 10 seeds, each model took 4-5 days to train on an Intel Xeon CPU E5-2697 v4 @ 2.30GHz. These were averaged over 10 gradient updates for each backpropagation step. We used an RMSProp optimizer with a learning rate of 0.003. 

% \subsection{Additional Environments: Predator-Prey}

% % \begin{figure}[!ht]
% %     \centering
% %     \includegraphics[width=\textwidth]{figs/predator_prey.png}
% %     \caption{Zoomed-in view of the $20 \times 20$ predator-prey environment. The predators are denoted by green aliens, while the prey is denoted by a human (in a red square).}
% %     \label{fig:pp_env}
% % \end{figure}

% \paragraph{Experiment Setup}
% % {Note that we do not train on SMAC~\cite{SMAC} as this benchmark has been shown to be fully solvable without communication~\cite{UPDeT}. Thus, sparse communication in such a task is trivial.}

% % The predator-prey scenario~\cite{commnet,ic3net} involves multiple agents, where one agent is denoted as the prey and the remaining agents are denoted as predators. The predator agents move and search the environment for the prey agent, which is stationary. Once the predator agent reaches the prey agent, it remains there for the remainder of the episode. The environment is composed of a $20 \times 20$ grid where each agent can occupy one cell, and the agents spawn at random cells at the beginning of each episode. Moreover, if the agent has not reached the prey agent, then the predator agent can choose to move to an adjacent cell at each time-step. Note that both communication and action occur in a single time-step. The predator agents can only observe its current cell and the adjacent cells (limited visibility to 1 cell around itself). The episode terminates when all predator agents reach the prey agent or when the maximum episode length is hit.

% % % Purpose of experiment
% % Unlike traffic junction, predator-prey does not necessarily require communication to solve the task. In the fully-cooperative predator-prey environment, predators are rewarded for the total number of predators who reach the discovered prey. Thus, there is no built-in incentive for fully-cooperative multi-agent teams to decrease total communication. In our experiments, we show that our method, IMGS-MAC, is able to decrease communication to a minimum budget $b^*$ with lossless performance.

% % \begin{figure}[!ht]
% %     \centering
% %     \includegraphics[width=.45\textwidth]{figs/pp_hard_baseline_autoencoder.png}
% %     \includegraphics[width=.45\textwidth]{figs/pp_hard_baseline_proto_autoencoder.png}
% %     \caption{Above compares the training IC3Net baseline (blue) vs. our IMGS-MAC (orange) with non-sparse communication ($b=1$). Our method converges to higher success earlier and with less variance.}
% %     \label{fig:pp_autoencoder}
% % \end{figure}





% % discussion of results
% First, we analyze the performance of our IMGS-MAC versus IC3Net baseline when trained with non-sparse communication $b=1$. With continuous communication, our method is able to find higher reward solutions due to its more informative communication, which occurs due to the use of the autoencoder. This is even more evident with discrete communication. See Figure~\ref{fig:pp_autoencoder}. 

% With informative emergent communication, we can remove redundant null communications. See Figure~\ref{tab:analytical_auto_pp}. However, since there are more states total in predator prey than traffic junction, while IMGS-MAC greatly reduces the redundant usage of communication vectors, we find that the usage of null communications with IMGS-MAC is higher in predator-prey than traffic junction. This may also have to do with encoding additional information besides the observation of the state into the communication vector.



% Finally, we show how are model exhibits few-shot and zero-shot sparsity. We perform PCA analysis to determine the threshold in which we can remove null communications and still retain task performance. In Table~\ref{table:lossless_pp}, we report the minimum lossless budget $b^*$. In Figure~\ref{fig:pp_budgets}, we show that the average report for our zero-shot sparsity ($b=b^*$) is truly lossless. While for budgets $b<b^*$, there is a tradeoff between reward and the suboptimal budget. It is interesting to note that in this fully-cooperative problem where communication is not necessarily required to complete the task, our model is able to greatly reduce the budget, which means that most of the performance does not require communication. It could be the case that we need to learn a method \textit{to rely more} on our informative communication to further increase performance.

% % \begin{table*}[!ht]
% % \centering
% %     \caption{Average $\mu \pm \sigma$ for quality and performance of null communication vectors. IMGS-MAC (ours) provides significantly more informative communication, as recognized by its low usage of null communications. Lower is better.}
% % \begin{tabularx}{\textwidth}{X X| X X X} 
% %  \specialrule{.2em}{.1em}{.1em} 
% %   \multirow{ 2}{*}{Environment} & \multirow{ 2}{*}{Method} & \% Null Comm. Vectors & \# Observations \newline per Vector & \% Null Comms. \newline Emitted\\
% %   \hline
% %     \multirow{ 2}{*}{PP Hard Cts.} &   IC3Net Baseline & 0.784 \small $\pm$ 0.0445 & 73.148 \small $\pm$ 12.099 & 0.497 \small $\pm$ 0.0887 \\ 
% %     & \textbf{IMGS-MAC} & 0.284 \small $\pm$ 0.160 & 17.523 \small $\pm$ 6.231 & 0.300 \small $\pm$ 0.173\\
% %     \hline
% %     \multirow{ 2}{*}{PP Hard Discrete} &  IC3Net Baseline & 0.482 \small $\pm$ 0.145 & 104.803 \small $\pm$ 6.0713 & 0.719 \small $\pm$ 0.312 \\
% %     & \textbf{IMGS-MAC} & 0.380 \small $\pm$ 0.0909 & 82.809 \small $\pm$ 6.507 & 0.141 \small $\pm$ 0.114  \\
    
% % \specialrule{.1em}{.05em}{.05em}
% % \end{tabularx}
% %     \label{tab:analytical_auto_pp}
% % \end{table*}

% % \begin{table}[!ht]
% % \centering
% % \caption{Minimum sparse budget $b^*$ with lossless performance, $\mu \pm \sigma$.}
% % \begin{tabularx}{\textwidth}{|X| X X|} 
% %  \specialrule{.2em}{.1em}{.1em} 
% %   Environment & PP Hard Cts. & PP Hard Discrete \\
% %   \hline 
% %   Min Budget $b^*$ & 0.244 \small $\pm$ 0.0644 & 0.263 \small $\pm$ 0.00757 \\
% % \specialrule{.1em}{.05em}{.05em}
% % \end{tabularx}
% % \label{table:lossless_pp}
% % \end{table}

% % \begin{figure}[!ht]
% %     \centering
% %     \includegraphics[width=.45\textwidth]{figs/lossless_success_pp_hard_continuous.png}
% %     \includegraphics[width=.45\textwidth]{figs/lossless_success_pp_hard_discrete.png}
% %     \caption{Success versus budget for IMGS-MAC at baseline non-sparse $b=1$, lossless $b=b^*$, and suboptimal $b<b^*$. Our model provides lossless performance for $b=b^*$ for $b^*$ in Table~\ref{table:lossless_pp} as compared with the baseline non-sparse $b=1$. Our performance tapers for smaller budgets until it approaches the no communication performance.}
% %     \label{fig:pp_budgets}
% % \end{figure}

% % \subsubsection{Starcraft II 3m}
% % {This experiment will help show the scale of our method}

% % \input{sections/08_appendix_A}
