# Supplementary material for: Towards True Lossless Sparse Communication in Multi-Agent Systems
Source: arXiv:2212.00115 source file (2022-11-30)
Supplement: Supplementary file 2 [file 08_appendix_A.tex]

% \subsection{On Reward-based Sparse Communication}\label{reward}
% We compare with an attempted stabilized version of ECNet that retains the sparsity benefits of ECNet as well as the performance benefits of IC3Net, which we call the Enforcers. We discuss the benefits and limitations of ECNet and IC3Net in section~\ref{related}. In this section, we present results from competing reward-based sparse communication methods. However, we find that this method still have issues with stability. Over running 10 seeds, only at most 3 converged to a budget. That is, we found that reward based methods are not able to follow a budget the other at least 7 times. Below, we present additional methodology used to attempt to increase the stability of reward-based sparse communication under a budget. Then we present experimental results in traffic junction and predator-prey methods with discrete communication. We emphasize that our presented method, IMGS-MAC, clearly outperforms the Enforcers in terms of stability, rendering additional comparisons inconsequential. Even so, we present the Enforcers to show the limits of reward-based sparse communication.


%  The Enforcers are a reward-based sparse communication method used to constrain communication for arbitrary budgets. To enable any convergence, we implement a communication curriculum. For each of the enforcers, the communication curriculum fixes an open gate, $b=1$, which allows unrestricted, non-sparse communication. %See figure \ref{fig:gateBlock}. 
%  After achieving a success criterion, the network learns a gating function with a reward function that penalizes any restriction on communication,
% $
%     R^i = R^i_{env} - \lambda R^i_{comm},
% $
% where, in this case,
% \begin{equation*}
%     R^i_{comm} = R^i_{commMax} = |1 - c_{AVG}^i|.
% \end{equation*} 
% After achieving the success criterion again with the new reward function, we allow The Enforcers to do their job to further constrain the communication. If $c_{AVG}$ is within some $\epsilon$ of our budget, the learning rate is tapered to enable convergence of the joint communication and action policy.

% % \begin{figure}[h]
% %     \centering
% %     \includegraphics[width=.3\textwidth]{figs/curriculum.png}
% %     \caption{Above shows each section of the curriculum used to train the Enforcers (left), including the conditions to enter the next phase of the curriculum (right). For the ``Open Gate'', which uses non-sparse communication ($b=1$), and ``Positive Communication Reward'', which learns to maximize communication, phases, the next phase is triggered by finding that the average reward is over a predefined threshold. Then, once the soft enforcer converges, the Enforcers checks if the observed $c_{AVG}$ is within an $\epsilon$-neighborhood of the budget. If it is, we finish training, otherwise we use the hard enforcer.}
% %     \label{fig:gateBlock}
% % \end{figure}

% \subsubsection{Soft Enforcer}
% The soft enforcer uses a tuned reward function to ensure that communication is within a budget. However, the soft enforcer allows the agent to exceed the budget as it sees fit. That is, there exists some $\epsilon_s$, we have, $|b-c_{AVG}|<\epsilon_s$, such that the $\epsilon_s$ is learned at the discretion of the model. We define a reward penalty proportional to a scaled distance to the proposed budget $b$,
% $
%     R^i_P = \begin{cases} 
%       \frac{b-c_{AVG}}{b} & c_{AVG} \leq b\\
%       \frac{b-c_{AVG}}{1-b} &  c_{AVG} > b
%    \end{cases},
% $
% We also incorporate a first-order derivative term, 
% $
%     R^i_D = R^i_P - R^{i-1}_P,
% $
% and an integral term, 
% $
%     R^i_I = \sum_{j=0}^i R^j_P,
% $
% to the communication penalty reward, 
% \begin{equation*}
%     R^i_{comm}  = R^i_{commSoft} = \lambda_P R^i_P + \lambda_D R^i_D + \lambda_I R^i_I.
% \end{equation*}
% The hyperparameters are tuned empirically. Note that the method limits the integral term such that $|R^i_I| < K$ for some hyperparameter $K$ for stability. Our experiments used $K=0.1$, $Kp=1$, $Kd=1.6$, and $Ki=0.026$.

% The defined reward has the effect of limiting the variance of the reward over an episode, which, in turn, provides a soft limit of the change in the gating action. However, since it is only a soft limit, it increases the complexity of the objective for the value function.

% \begin{table}[!t]
% \centering
% \caption{\textbf{Traffic Junction:} The table above shows the results of training using the soft enforcer with different budgets $b$. We compare the $c_{AVG}$ $\backslash$ success rate for each budget. When successfully converged, the soft enforcer is able to follow the budget with a tradeoff between budget and performance. However, the Enforcers are only able to converge at most 30\% of the time, while IMGS-MAC converges 100\% of the time with lossless performance.}
% \begin{tabularx}{\textwidth}{c|X X}
% \specialrule{.2em}{.1em}{.1em}
% \multicolumn{3}{c}{\textbf{Soft Enforcer ($c_{AVG}$ $\backslash$ Success \% $\backslash$ Convergence \%)}}\\
%  \specialrule{.2em}{.1em}{.1em}
%   \textbf{Budget} &  \textbf{Easy} &  \textbf{Medium} \\
%  \hline
%  1 & 1.00 $\backslash$ .993 $\backslash$ 1 & 1.00 $\backslash$ .959 $\backslash$ 1 \\
%  .9 & .889 $\backslash$ .983 $\backslash$ .3 & .883 $\backslash$ .955 $\backslash$ .3 \\ 
%  .7 &  .781 $\backslash$ -----  $\backslash$ .1 &  .682 $\backslash$ .946 $\backslash$ .3 \\
%  .5 & .588 $\backslash$ ----- $\backslash$ .1  & .445 $\backslash$ .947 $\backslash$ .3 \\ %[1ex] 
%  .3 & .282 $\backslash$ ----- $\backslash$ .1  & .261 $\backslash$ .931 $\backslash$ .3 \\
% \specialrule{.1em}{.05em}{.05em}
% \end{tabularx}

% \label{table:tj_soft}
% \end{table}

% \subsubsection{Reward-based Sparsity Experiments}

% In this section, we show results for the reward-based Enforcers in traffic junction with discrete communication. We only present values for the Enforcers which converge for at least 3 seeds over the 10 seeds in which we experimented. Though the curriculum for the Enforcers helps stabilize the performance of reward-based sparsity, our method, IMGS-MAC clearly outperforms the Enforcers in terms of stability.



% The results for the soft enforcer show that the method is able to follow the budgets with a tradeoff with task performance. However, even in these cases, convergence is often poor. The soft enforcer does not necessarily follow the budget and trivially converges to $b=1$. Table \ref{table:tj_soft} shows the results of the soft enforcer with different values of the budget $b$, showing the performance for the best seed. For the easy traffic junction environment, the model is only able to converge over 30\% of the time when $b\geq .9$. For the medium traffic junction environment, we observe a tradeoff between task performance and the converged budget. Overall, the Enforcers are unable to converge to ultra-low levels of communication due to their suboptimal nature, which contradicts the joint communication and task performance reward.
% Our proposed method, IMGS-MAC, is able to converge 100\% of the time in scenarios for all $b$, while also performing losslessly with $b\geq b^*$ as shown in section~\ref{experiments}.


 
